# Supplementary material for: Quantum transport through pairs of edge states of opposite chirality at electric and magnetic boundaries
Source: arXiv:1803.11452 source file (2018-03-30)
Supplement: Supplementary file 1 [file supple_final.pdf]

# Quantum transport through pairs of edge states of opposite chirality at electric and magnetic boundaries

Puja Mondal[1], Alain Nogaret[2] and Sankalpa Ghosh[1]

[1] *Department of Physics, Indian Institute of Technology Delhi, New Delhi-110016, India and*

[2]*Department of Physics, University of Bath, Bath BA2 7AY, UK*

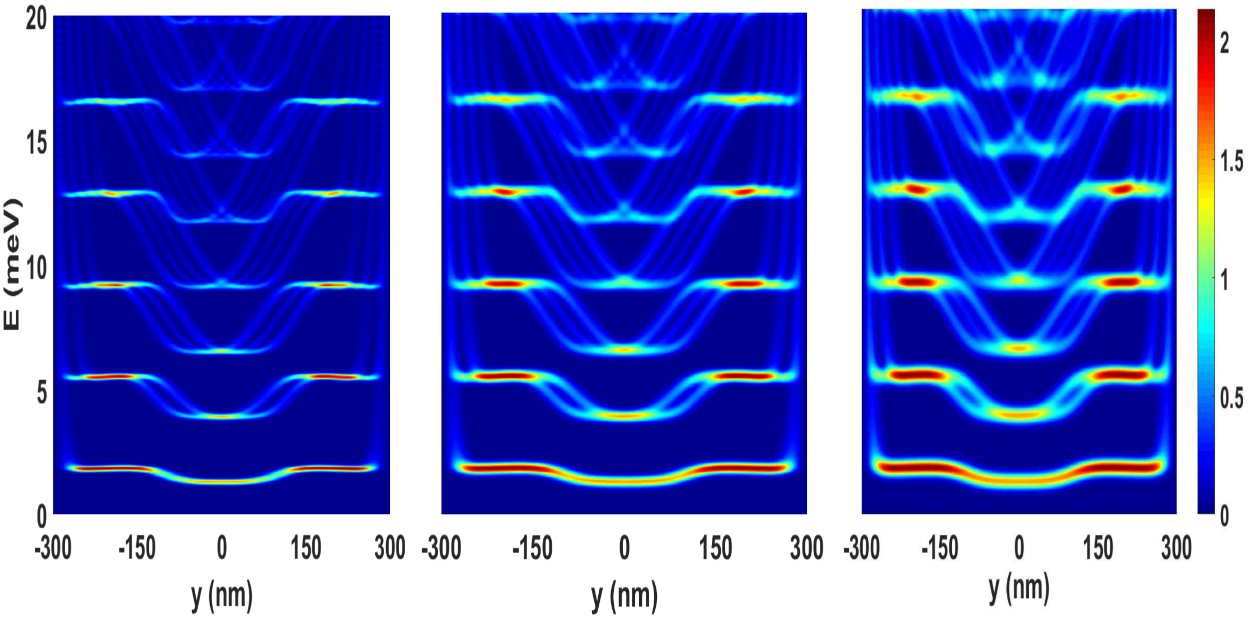


FIG. 1: *(color online)* LDOS at $B_a$=2 T and for $W_e$=600 nm in the magnetic split gate for $\Gamma$=0.1 meV, 0.2 meV and 0.3 meV.

## I. LDOS FOR WEAKER BROADENING

Fig. 1 shows the local density of states for weaker impurity broadening $\Gamma$=0.1 meV, 0.2 meV and 0.3 meV. The LDOS shows that the splitting depends on the number of nodes in the wavefunction. As $\Gamma$ increases, the splitting gets blurred in the LDOS. Also, LDOS clearly represents the fact that the magnetic minibands of the higher Landau levels overlap with each other.

## II. BAND AND NON-DIAGONAL CONDUCTIVITY

We have calculated the diagonal component of the diffusion conductivity using

$$\sigma^d_{xx} = \frac{\beta e^2}{A}\sum_{n,k_x}\int dE\ P(E-E_{n,k_x})f(E)(1-f(E))\tau|\upsilon^n_x(k_x)|^2 \tag{II.1}$$

where $P(E-E_{n,k_x})$, $\tau(E)$ and A are the Gaussian broadening induced by the impurity, momentum relaxation time and area of the sample. The impurity broadening is of the form $P(E-E_{n,k_x}) = \frac{1}{\Gamma\sqrt{\pi}}exp\left(-\frac{(E-E_{n,k_x})^2}{\Gamma^2}\right)$, $\Gamma$ being the energy broadening We have shown the band conductivity in Fig. 2 in the split and strip gate. The band conductivity shows similar behaviour as a function of applied magnetic field $B_a$ in the two magnetic gates. The

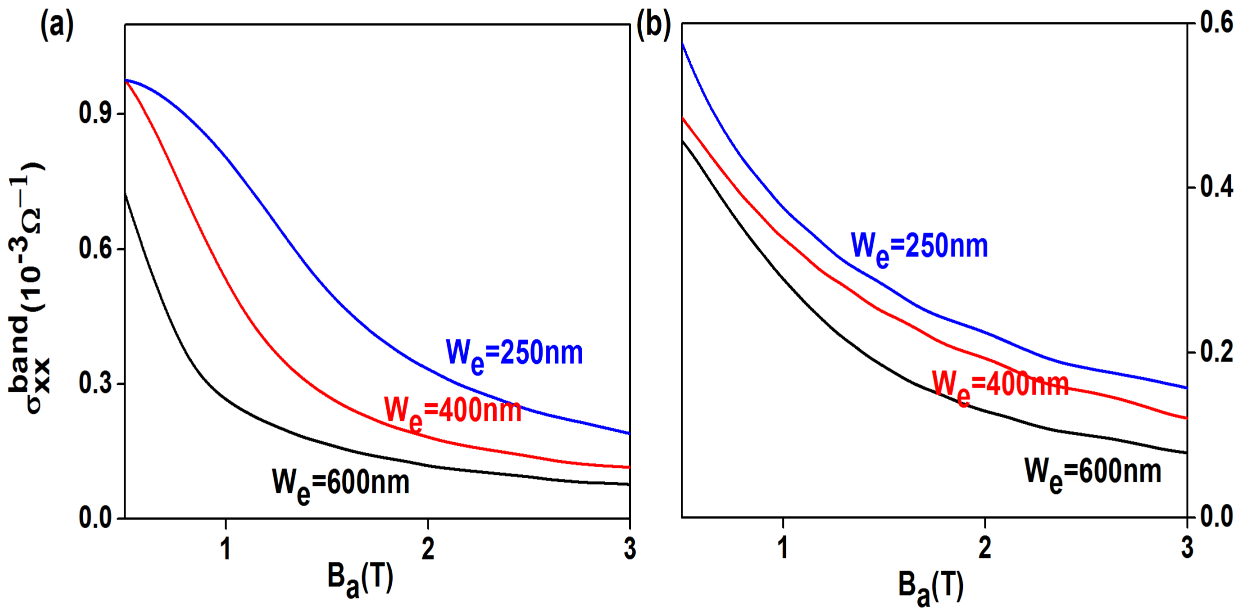


FIG. 2: *(color online)* Band conductivity vs applied magnetic field for decreasing channel width in the split (a) and magnetic strip (b) gate.

band band conductivity decreases as $B_a$ increases due to decreasing group velocity of the magnetic edge states. The non-diagonal component of the conductivity tensor is plotted in Fig. 3. The non diagonal diffusion conductivity is given by

$$\sigma_{\mu\nu}^{nd} = \frac{i\hbar e^2}{A} \sum_{\xi \neq \xi'} \frac{f_\xi (1 - f_{\xi'}) \langle \xi | v_\mu | \xi' \rangle \langle \xi' | v_\nu | \xi \rangle}{E_\xi - E_{\xi'}} \frac{1 - e^{\beta(E_\xi - E_{\xi'})}}{E_\xi - E_{\xi'}}$$

Using the identity $f_\xi(1-f_{\xi'})(1-e^{\beta(E_\xi - E_{\xi'})}) = f_\xi - f_{\xi'}$, the non diagonal conductance becomes

$$\begin{aligned} \sigma_{yx}^{nd} &= \frac{i\hbar e^2}{A} \sum_{\xi \neq \xi'} \frac{\langle \xi | v_y | \xi' \rangle \langle \xi' | v_x | \xi \rangle}{(E_\xi - E_{\xi'})^2} [f_\xi - f_{\xi'}] \\ &= \frac{e^2}{hL_y} \sum_{n \neq n'} \int dk_x [f_\xi' - f_\xi] \Big( \langle n, k_x | \hat{y} | n', k_x \rangle \langle n', k_x | \hat{x} | n, k_x \rangle \Big) \end{aligned} \qquad \text{(II.2)}$$

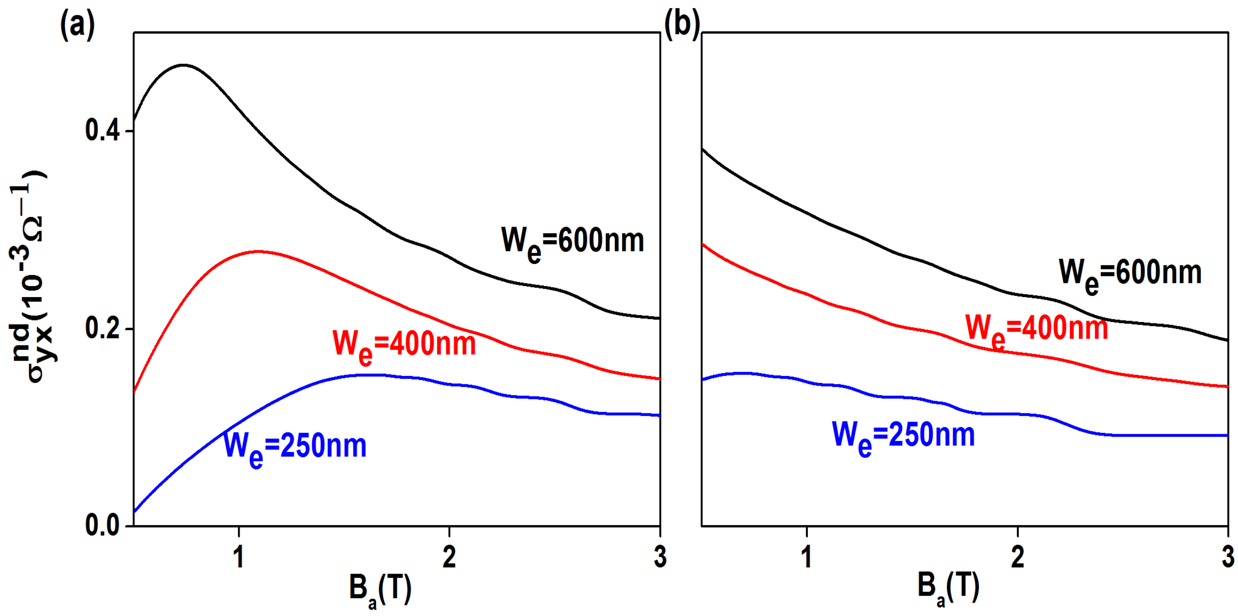


FIG. 3: *(color online)* Non-diagonal conductivity as a function of applied magnetic field for decreasing channel width in the split (a) and strip (b) gate. Curves are offset vertically for clarity.
